# Supplementary material for: CREIMBO: Cross-Regional Ensemble Interactions in Multi-view Brain Observations
Source: arXiv:2405.17395 source file (2025-01-12)
Supplement: Supplementary file 1 [file supplementary_technical_details.tex]

\section{Code and Data Sharing}\label{sec:data_code}
The neural data used in this study~\cite{kyzar2024dataset} is publicly available  with License: ``spdx:CC-BY-4.0''. We used version 0.240123.1806 of the data which can be accessed through the DANDI Archive at \url{https://dandiarchive.org/dandiset/000469/0.240123.1806} (Access Information: dandi:OpenAccess). 
The code will be shared on GitHub upon publication. 

\section{Technical Details}\label{sec:technical}
The whole code is written in Python. We utilized the following Python packages along with their respective versions: scipy (1.8.0), matplotlib (3.8.2), numpy (1.23.5), pandas (1.5.0), seaborn (0.11.2), scikit-learn (1.0.2), pylops (1.18.2), and statsmodels (0.13.2), all within a Python 3.10.4 environment. For the $\ell_1$ regularization, we used the ``SPGL1'' solver of pylops~\cite{van2009probing}.  %Sample of the data (e.g. ~5 sessions, with ~400 time points each) can run on a simple desktop machine however higher data might require additional processing. 
During the writing process, we used ChatGPT very sparingly to improve wording and fix grammar mistakes at the word or sentence level.
The synthetic experiment can run locally on a desktop (e.g., simple ASUS machine). However, the robustness tests with hundreds of random repeats and the human data experiments used the entry node with CPUs only of NERSC's ``Perlmutter'' supercomputer. Running time for each synthetic instance ranges from 0.8 to 2 minutes (with the capability to run in parallel). For the human data, processing all 41 sessions with 1000 time points per session (and varying neuron counts as described in the text and figures) takes between 17 to 25 minutes, depending on parameters and result quality.
